# Supplementary material for: Operation of an archaeological lead PbWO$_4$ crystal to search for neutrinos from astrophysical sources with a Transition Edge Sensor
Source: arXiv:2111.07638 source file (2021-11-15)
Supplement: Supplementary file 1 [file JLTP_SI_template_LTD18.pdf]

## Title

**A.B. Name · C.D. Name**

the date of receipt and acceptance should be inserted later

**Abstract** Insert abstract text directly after the heading. Leave an empty line after the abstract. Abstract should be one paragraph, with no indentation, and justified.

**Keywords** keyword 1, keyword 2...

### 1 Section Title

When preparing your manuscript, please follow the instructions in this template. This template serves as a universal template for Special Issue Articles to be taken into consideration for publication in the Journal of Low Temperature Physics.

Insert an empty line after the section title. Indent at the start of each paragraph after the first paragraph of the section, which is not indented. For special issue articles the page length is 6 pages. Invited contributions may be 12 pages long. In order to estimate your article length, please prepare your manuscript in Times or Times New Roman, font size 11, justify the body text, and make sure the page format is set to A4. The template margins are: Top: 2.07, Left: 1.77, Bottom: 2.17, Right: 1.77 inches.

Subsections can be used.

### 2 Section Title

#### 2.1 Equations

Place equations in the text and number them, for example:

$$\frac{\rho - \rho_0}{\rho_0} = aH + bH^2, \quad (1)$$

---

Department of Physics, Name University,  
City, STATE zip, Country  
Tel.:  
Fax:  
E-mail: name@email.com

**Fig. 1** Insert the figure caption directly after the header. Use the words *Top*, *Bottom*, *Left*, and *Right* (in italics) to denote the sub figures being described. Additional annotation should also be in italics, e.g., *solid symbols*, *open symbols*, *red*, *dashed line*, etc. If including color figures, please supply a B&W or greyscale figure as well for print and include the following statement at the end of your caption: (Color figure online.)

When referring to equations please use parentheses and the number of the equation as follows: Eq. (1).

## 2.2 Figures

When inserting figures, Leave an empty line after the Figure caption. When referring to figures in the text, please do so as follows: Fig. 2.

## 3 Section Title

### 3.1 References

Regarding references: please see the example bibliography below. Please include DOI numbers wherever possible. Please number your references in order of appearance in the text. Citations should be with square brackets as follows [1], [2,3] or [4-7]. Please use the commonly used and accepted journal abbreviation whenever possible. For example, the Journal of Low Temperature Physics is J. Low Temp. Phys.

When citing articles that shall appear in the same special issue, please do the following. During the review stage you will be asked to cite the article as A. Name, J. Low Temp. Phys. This Special Issue (YEAR). Upon acceptance of the article and receiving the proofs, you will be requested to update the references and replace "This Special Issue" with the full citation and DOI number. Articles that have been accepted and published online (on SpringerLink) will immediately have a DOI number even if they are not assigned to an issue yet. When citing articles that appeared in previous special issues of this journal, please use the standard citation and include the DOI number.

**Acknowledgements** (Optional) Please enter text directly after the header. Template v.1 by KLL - June 18, 2015.

---

**References**

1. R. Joynt and L. Taillefer, *Rev. Mod. Phys.* **74**, 235, (2002), DOI:10.1103/RevModPhys.74.235.
2. J.B. Kycia, J.I. Hong, M.J. Graf, J.A. Sauls, D.N. Seidman, and W.P. Halperin, *Phys. Rev. B* **58**, R603, (1998), DOI:...
3. R.H. Heffner, D.W. Cooke, A.L. Giorgi, R.L. Hutson, M.E. Schillaci, H.D. Rempp, J.L. Smith, J.O. Willis, D.E. MacLaughlin, C. Boekema, R.L. Lichti, J. Oostens, and A.B. Denison, *Phys. Rev. B* **39**, 11345, (1989), DOI:...
4. G. Aeppli, E. Bucher, C. Broholm, J.K. Kjems, J. Baumann, and J. Hufnagl, *Phys. Rev. Lett.* **60**, 615, (1988).
5. P. Dalmas de Réotier, A. Huxley, A. Yaouanc, J. Flouquet, P. Bonville, P. Imbert, P. Pari, P.C.M. Gubbens, and A.M. Mulders, *Phys. Lett. A* **205**, 239, (1995).
6. R.A. Fisher, B.F. Woodfield, S. Kim, N.E. Phillips, L. Taillefer, A.L. Giorgi, and J.L. Smith, *Solid State Commun.* **80**, 263, (1991).
7. H. Tou, Y. Kitaoka, K. Asayama, N. Kimura, Y. Ōnuki, E. Yamamoto, and K. Maezawa, *Phys. Rev. Lett.* **77**, 1374, (1996).
8. K. Behnia, O. Laborde, L. Taillefer, and J. Flouquet, *Physica B* **165 & 166**, 431, (1990).
9. M. Lee, G.F. Moores, Y.-Q. Song, W.P. Halperin, W.W. Kim, and G.R. Stewart, *Phys. Rev. B* **48**, 7392, (1993).
10. J. Flouquet, *Progress in Low Temp. Phys.* **15**, 139, (2005).
11. E.A. Schuberth, B. Strickler, and K. Andres, *Phys. Rev. Lett.* **68**, 117, (1992).
12. J.P. Brison, N. Keller, P. Lejay, J.L. Tholence, A. Huxley, N. Bernhoeft, A.I. Buzdin, B. Fåk, J. Flouquet, L. Schmidt, A. Stepanov, R.A. Fisher, N. Phillips, and C. Vettier, *J. Low Temp. Phys.* **95**, 145, (1994).
13. S. Schöttl, E.A. Schuberth, K. Flachbart, J.B. Kycia, J.I. Hong, D.N. Seidman, W.P. Halperin, J. Hufnagl, and E. Bucher, *Phys. Rev. Lett.* **82**, 2378, (1999).
